# Supplementary material for: Making the Unaccountable Internet: The Changing Meaning of Accounting in the Early ARPANET
Source: arXiv:2201.11884 source file (2022-05-11)
Supplement: Supplementary file 4 [file appendix.tex]

\appendix

\input{sections/appendix/endnotes}

\input{sections/appendix/1researchservice}

\input{sections/appendix/2abbateusability}

\input{sections/appendix/3methods}
