# Supplementary material for: Making the Unaccountable Internet: The Changing Meaning of Accounting in the Early ARPANET
Source: arXiv:2201.11884 source file (2022-05-11)
Supplement: Supplementary file 5 [file endnotes.tex]

\theendnotes
